# Supplementary material for: MIGRO: A Decoupled and Portable Long-Term Memory System for Language Models
Source: arXiv:2611.15315 source file (2026-11-13)
Supplement: Supplementary file 1 [file storage_additional.tex]

\FloatBarrier
\section{Additional LoCoMo Storage Results}
\label{sec:storageadditional}
The ten matched conversations provide a shorter-history view of continued writing. At each prefix, Figure~\ref{fig:locomogrowth} compares the same eligible conversations; their count decreases with length. Figure~\ref{fig:locomomarginal} measures byte increments within each conversation before averaging. MIGRO's second-half cost is 4.207 bytes/token, versus 8.847 for LSTMem, 49.385 for TiMem, 113.668 for A-MEM, 410.676 for PlugMem, and 820.634 for Mem0. These measurements complement the matched-state quality comparison in Section~\ref{sec:storage}.

\begin{figure}[H]
\centering
\includegraphics[width=.87\linewidth]{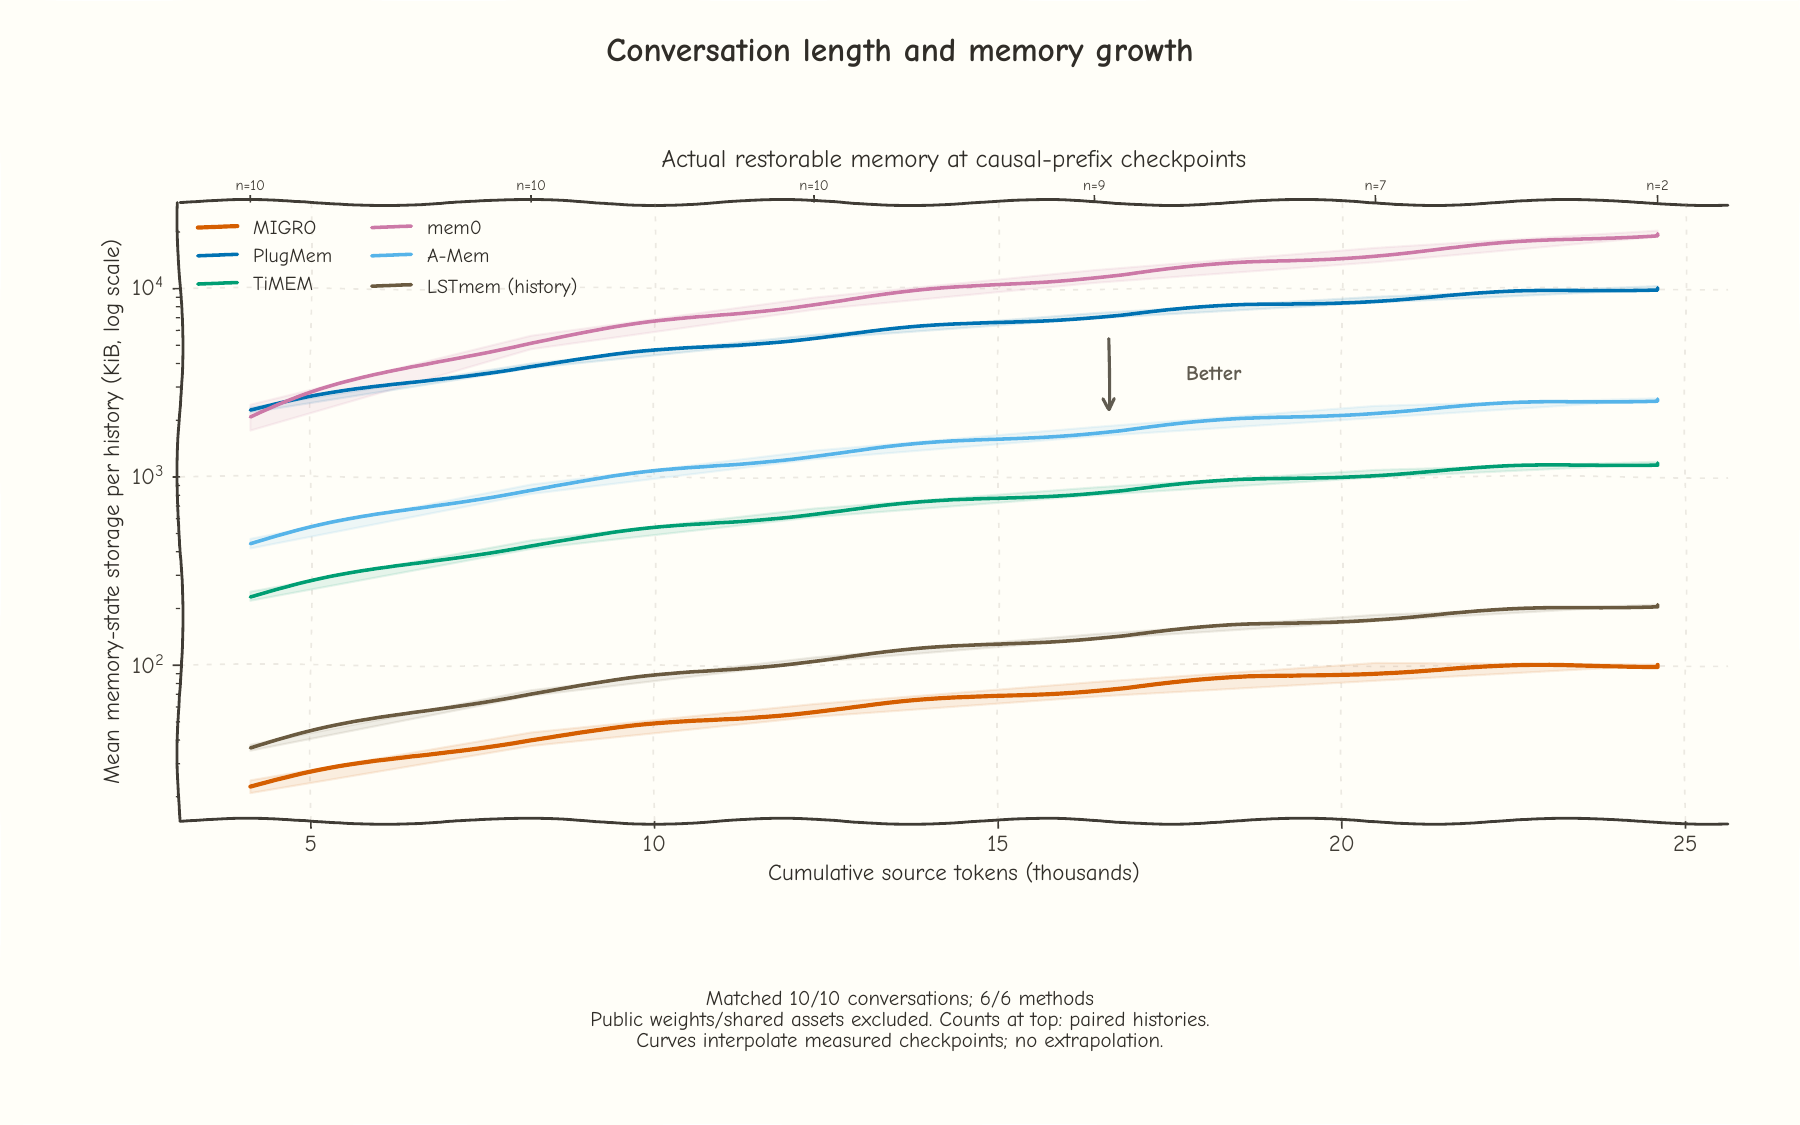}
\caption{LoCoMo native memory growth across the same eligible conversations at each prefix. Counts above the plot show the available natural histories.}
\label{fig:locomogrowth}
\end{figure}

\begin{figure}[H]
\centering
\includegraphics[width=.87\linewidth]{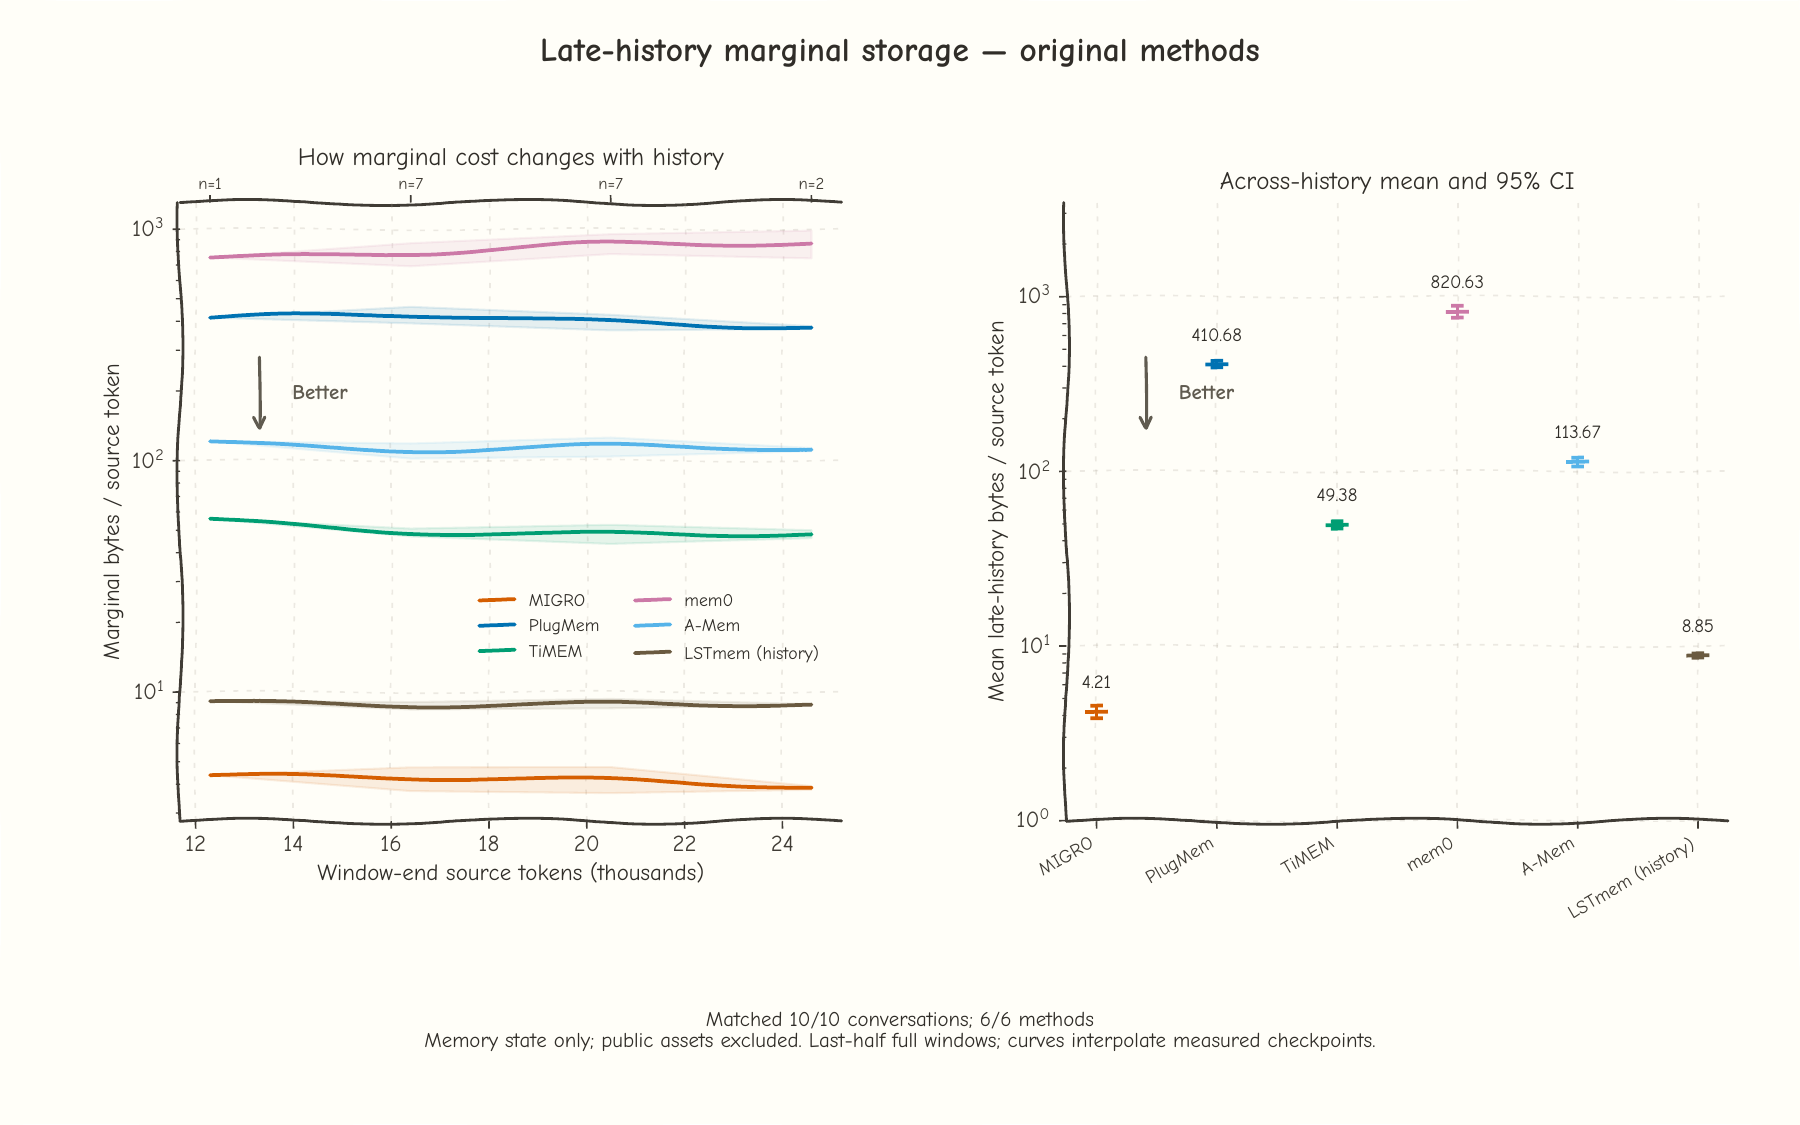}
\caption{LoCoMo incremental storage. Left: later-history windows. Right: mean second-half cost and 95\% conversation-bootstrap intervals; MIGRO averages 4.207 bytes/token.}
\label{fig:locomomarginal}
\end{figure}
\FloatBarrier
